# Supplementary material for: A probabilistic, data-driven closure model for RANS simulations with aleatoric, model uncertainty
Source: arXiv:2307.02432 source file (2024-04-15)
Supplement: Supplementary file 1 [file adjoint.tex]

++++++++++++++

++++++++++++++++

In order to  embed the RANS solver in the computational graph and thus perform model-based training, we advocate the use of discrete, adjoint  methods \cite{giles2000introduction}.
%for solver gradients as it will facilitate learning using state of the art deep learning methods \cite{lecun2015deep}. 
In effect it will connect the discretized RANS solver  with the auto-differentiation  tools \cite{baydin2018automatic} of the modern machine learning libraries \cite{paszke2017automatic} thus enabling end-to-end gradient flow. The approach is computationally efficient, especially for the current scenario as the cost of obtaining the gradients is independent of the number of parameters and the parametric fields $\tauTheta$, $\epsTau$.  This is very useful here as the dimension of the RS field can scale with the mesh resolution.
%potentially has many degree of freedom corresponding to the mesh resolution. 
However the intrusive nature of adjoints presents a major challenge in the development process. 
%This study employs discrete adjoint technique to calculate the gradient of the ELBO $\mathcal{F}$ (\refeq{eq:ELBO}) w.r.t the parameters. Its important to highlight that the cost of computing the gradients are independent of the number of parameters. This is very useful here as the dimension of the RS field can scale with the mesh resolution. 

For the likelihood given by $\ell$, firstly, a Lagrangian $\calL$ with the Lagrangian multiplier $\lambda$ is introduced given by, 

\begin{align}
	\calL=\ell + \bm \lambda^T(\calG(\bm{z})-\calB\bm{\tau})
\end{align}
where $\calG$, $\calB$, $\tau$ and $\z$ are as defined in \refsec{sec:methods}. Now the gradients w.r.t the parameters $\tau$ is evaluated and with the product rule given as,

\begin{align}
	\frac{d\calL}{d\bm{\tau}}&= \frac{\partial \ell}{\partial \bm{z}} \frac{d \bm{z}}{d\bm{\tau}} + \frac{d \bm \lambda^T}{d\bm{\tau}} (\calG(\bm{z})-\calB\bm{\tau}) + \bm \lambda^T \left(\frac{\partial \calG}{\partial \bm{z}} \frac{d \bm{z}}{d\bm{\tau}} - \calB\right)\nonumber \\
	&= \left(\frac{\partial \ell}{\partial \bm{z}} + \bm \lambda^T\frac{\partial \calG}{\partial \bm{z}} \right)\frac{d \bm{z}}{d \bm{\bm{\tau}}} - \bm \lambda^T \calB
	\label{eq:adjoint_expanded}
\end{align}

The additional degree of freedom introduced by the Lagrangian is used to assert that the expression in the parenthesis above must vanish. This leads to the following equation

\begin{align}
	\frac{\partial \ell}{\partial \bm{z}} + \bm \lambda^T\frac{\partial \calG}{\partial \bm{z}} = 0 \quad \textrm{or,} \quad \left(\frac{\partial \calG}{\partial \bm{z}} \right)^T \bm \lambda = - \left(\frac{\partial \ell}{\partial \bm{z}} \right)^T
\end{align}
for the Lagrangian multiplier or the so called adjoints ($\bm \lambda$) with $\text{dim}(\bm \lambda) = \text{dim}(\z)$ . They can be understood as a dual to the state variables $\bm u$ and $p$ here. For example, for RANS, the solution is a tuple of $\bm u$ and $p$, the adjoint $\bm \lambda$ is the tuple of adjoint velocity and pressure.
The linear system is solved by a direct LU solver, then the results is substituted back in \refeq{eq:adjoint_expanded} to obtain the desired gradients given by
\begin{align} \label{eq:Adjoint_gradient}
	\frac{d\calL}{d\bm{\tau}} = - \bm \lambda^T \calB
\end{align}

% We are interested in the decomposed representation of the RS presented in \refeq{eq:taudecomp}. Based on the formulation presented above, it is trivial to obtain the the gradients w.r.t the two terms $\tauTheta$ and $\epsTau$. They are given as

% \begin{align} 
% 	\frac{d\calL}{d\bm{\tauTheta}} = - \lambda^T \calB\\
% 	\frac{d\calL}{d\bm{\epsTau}} = - \lambda^T \calB
% \end{align}
